# Supplementary material for: Intrapapillary Capillary Loop Classification in Magnification Endoscopy: Open Dataset and Baseline Methodology
Source: arXiv:2102.09963 source file (2021-02-19)
Supplement: Supplementary file 1 [file appendix.tex]

\section{Number of patients and frames per fold}
\label{sec:appendix_dataset_numbers}
The number of patients per fold is shown in appendix table \ref{tab:folds_patients}. Similarly, the number of frames is shown in appendix table \ref{tab:folds_frames}.

\begin{table*}[!htbp]
	\centering
	\caption{Number of patients per fold (80\% training, 10\% validation, 10\% testing).}
	\begin{tabular}{lccccc}
		\hline
		\multicolumn{1}{c}{\bfseries Dataset} &
		\multicolumn{1}{c}{\bfseries Fold $1$} &
		\multicolumn{1}{c}{\bfseries Fold $2$} &
		\multicolumn{1}{c}{\bfseries Fold $3$} &
		\multicolumn{1}{c}{\bfseries Fold $4$} &
		\multicolumn{1}{c}{\bfseries Fold $5$} \\
		\hline
		Training (normal)              &  $36$ &  $35$ &  $39$ &  $36$  &  $36$ \\
		Training (abnormal)            &  $55$ &  $56$ &  $52$ &  $55$  &  $55$ \\
		Training (normal + abnormal)   &  $91$ &  $91$ &  $91$ &  $91$  &  $91$ \\
		\hline
		Validation (normal)            &  $5$  &  $6$  &  $2$  &  $5$   &  $6$  \\
		Validation (abnormal)          &  $6$  &  $5$  &  $9$  &  $6$   &  $5$  \\
		Validation (normal + abnormal) &  $11$ &  $11$ &  $11$ &  $11$  &  $11$ \\
		\hline
		Testing (normal)               &  $4$  &  $4$  &  $4$  &  $4$   &  $3$  \\
		Testing (abnormal)             &  $8$  &  $8$  &  $8$  &  $8$   &  $9$  \\
		Testing (normal + abnormal)    &  $12$ &  $12$ &  $12$ &  $12$  &  $12$ \\
	\end{tabular}
	\vspace{0.2cm}
	\label{tab:folds_patients}
\end{table*}
\begin{table*}[!htbp]
	\centering
	\caption{Number of frames per fold.}
	\begin{tabular}{lccccc}
		\hline
		\multicolumn{1}{c}{\bfseries Dataset} &
		\multicolumn{1}{c}{\bfseries Fold $1$} &
		\multicolumn{1}{c}{\bfseries Fold $2$} &
		\multicolumn{1}{c}{\bfseries Fold $3$} &
		\multicolumn{1}{c}{\bfseries Fold $4$} &
		\multicolumn{1}{c}{\bfseries Fold $5$} \\
		\hline
		Training (normal)               &  $22857$  &  $22883$  &  $23467$  &  $20504$  &  $24671$ \\
		Training (abnormal)             &  $33160$  &  $31959$  &  $33024$  &  $34905$  &  $28233$ \\
		Training (normal + abnormal)    &  $56017$  &  $54842$  &  $56491$  &  $55409$  &  $52904$ \\
		\hline
		Validation (normal)             &  $2667$   &  $3534$   &  $1649$   &  $4793$   &  $2781$  \\
		Validation (abnormal)           &  $2522$   &  $3883$   &  $4334$   &  $1500$   &  $3237$  \\
		Validation (normal + abnormal)  &  $5189$   &  $7417$   &  $5983$   &  $6293$   &  $6018$  \\
		\hline
		Testing (normal)                &  $2555$   &  $1662$   &  $2963$   &  $2782$   &  $627$   \\
		Testing (abnormal)              &  $3981$   &  $3821$   &  $2305$   &  $3258$   &  $8193$  \\
		Testing (normal + abnormal)     &  $6536$   &  $5483$   &  $5268$   &  $6040$   &  $8820$  \\
	\end{tabular}
	\vspace{0.2cm}
	\label{tab:folds_frames}
\end{table*}

\newpage
\section{Qualitative classification results and cases of patient failure}
%\section{Cases of patient failure}
%\section{Qualitative classification results for all folds}
%
\begin{figure*}[!h]
    \centering
    \includegraphics[width=\textwidth]{}
    \caption{Qualitative results for ResNet-18-CAM-DS on frame classification over the testing set of each fold. TP, TN, FP, FN stand for true positives, true negatives, false positives and false negatives respectively.
    \textit{Best} TP refers to the abnormal image with the highest estimated probability of being abnormal. Analogously, the \textit{best} TN represents the image with lowest estimated probability. Median and worst cases are estimated in a similar fashion. The FP median and worst case of fold $5$ are the same image because in the testing set of this fold there is only this false positive image.
    }
    \label{fig:qualitative_supervised_results}
\end{figure*}
\begin{figure*}[!h]
	\centering
	\includegraphics[width=\textwidth]{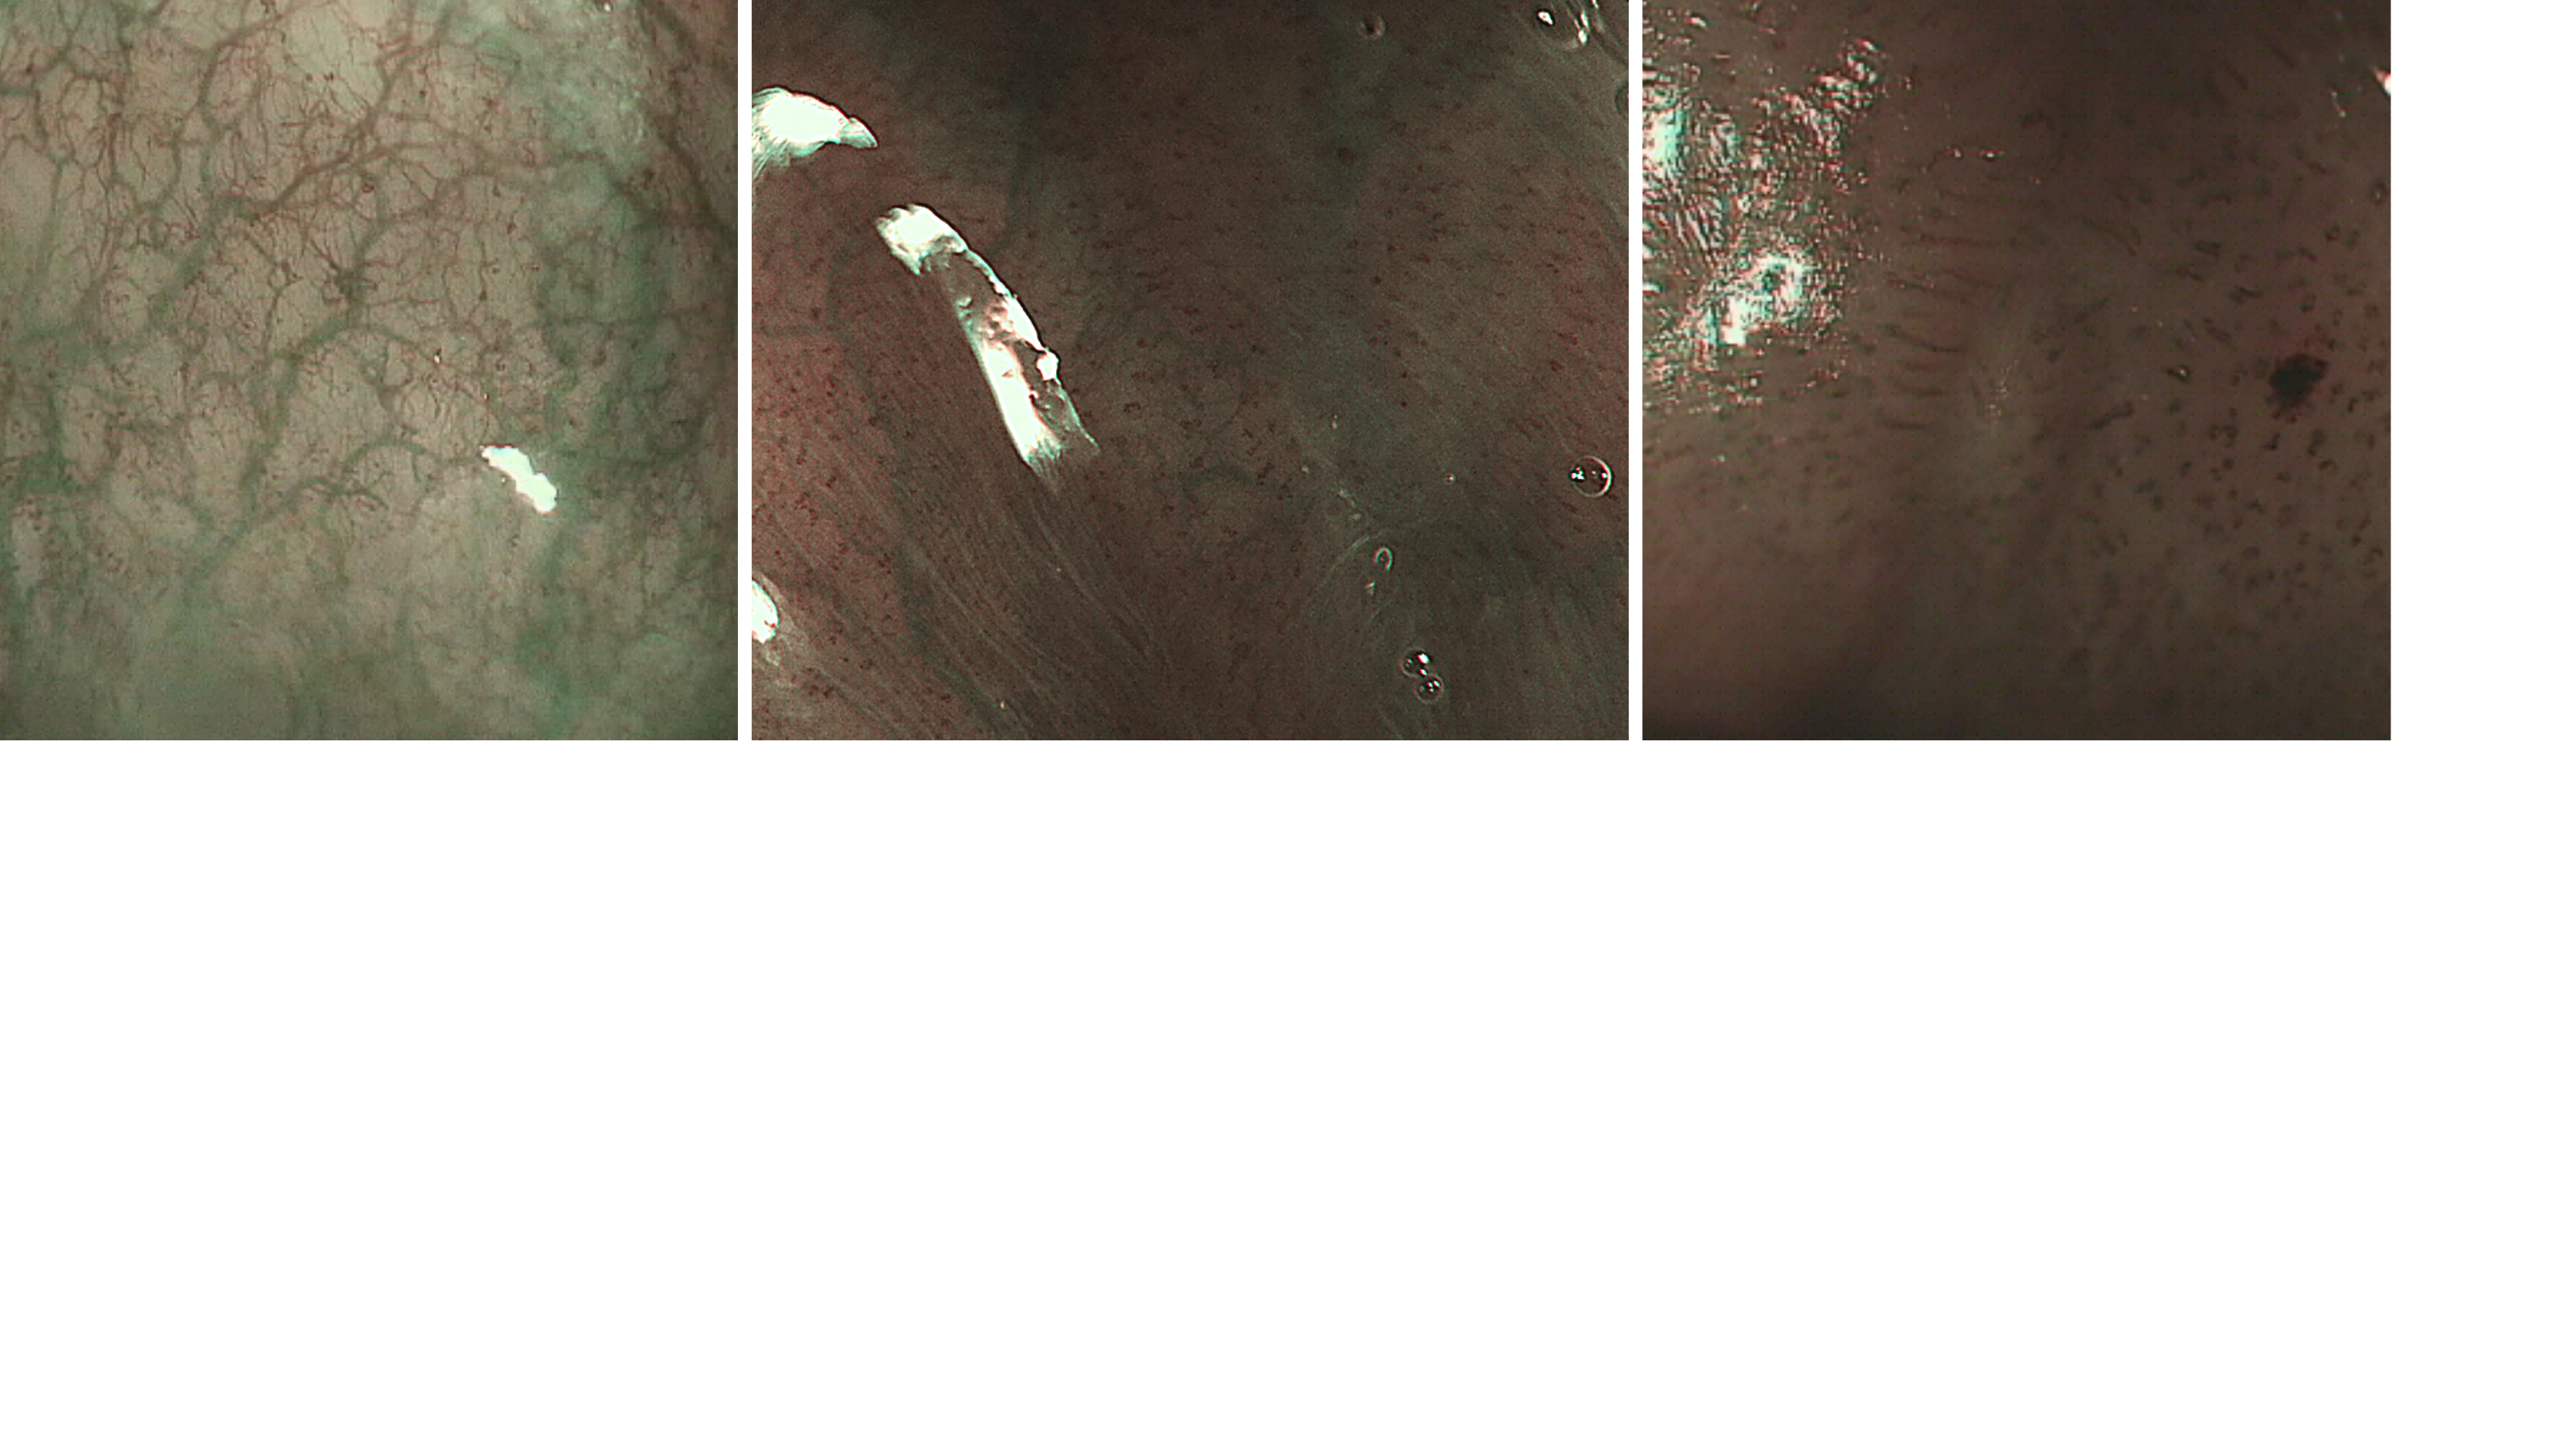}
	\caption{Representative frames of cases of patient failure (i.e. when the average estimated class for the whole patient clip is wrong). Patient $158$ (normal IPCL, left), $143$ (normal IPCL, center), $66$ (right, abnormal IPCL). ResNet-18 failed on all of them. ResNet-18-CAM only on $143$ and $66$. ResNet-18-CAM-DS failed only on case $158$.}
	\label{fig:patient_failure}
\end{figure*}

\newpage
\newpage

\section{ROC result for ResNet-18-CAM-DS}
\begin{figure*}[!h]
	\centering
	\includegraphics[width=0.9\textwidth]{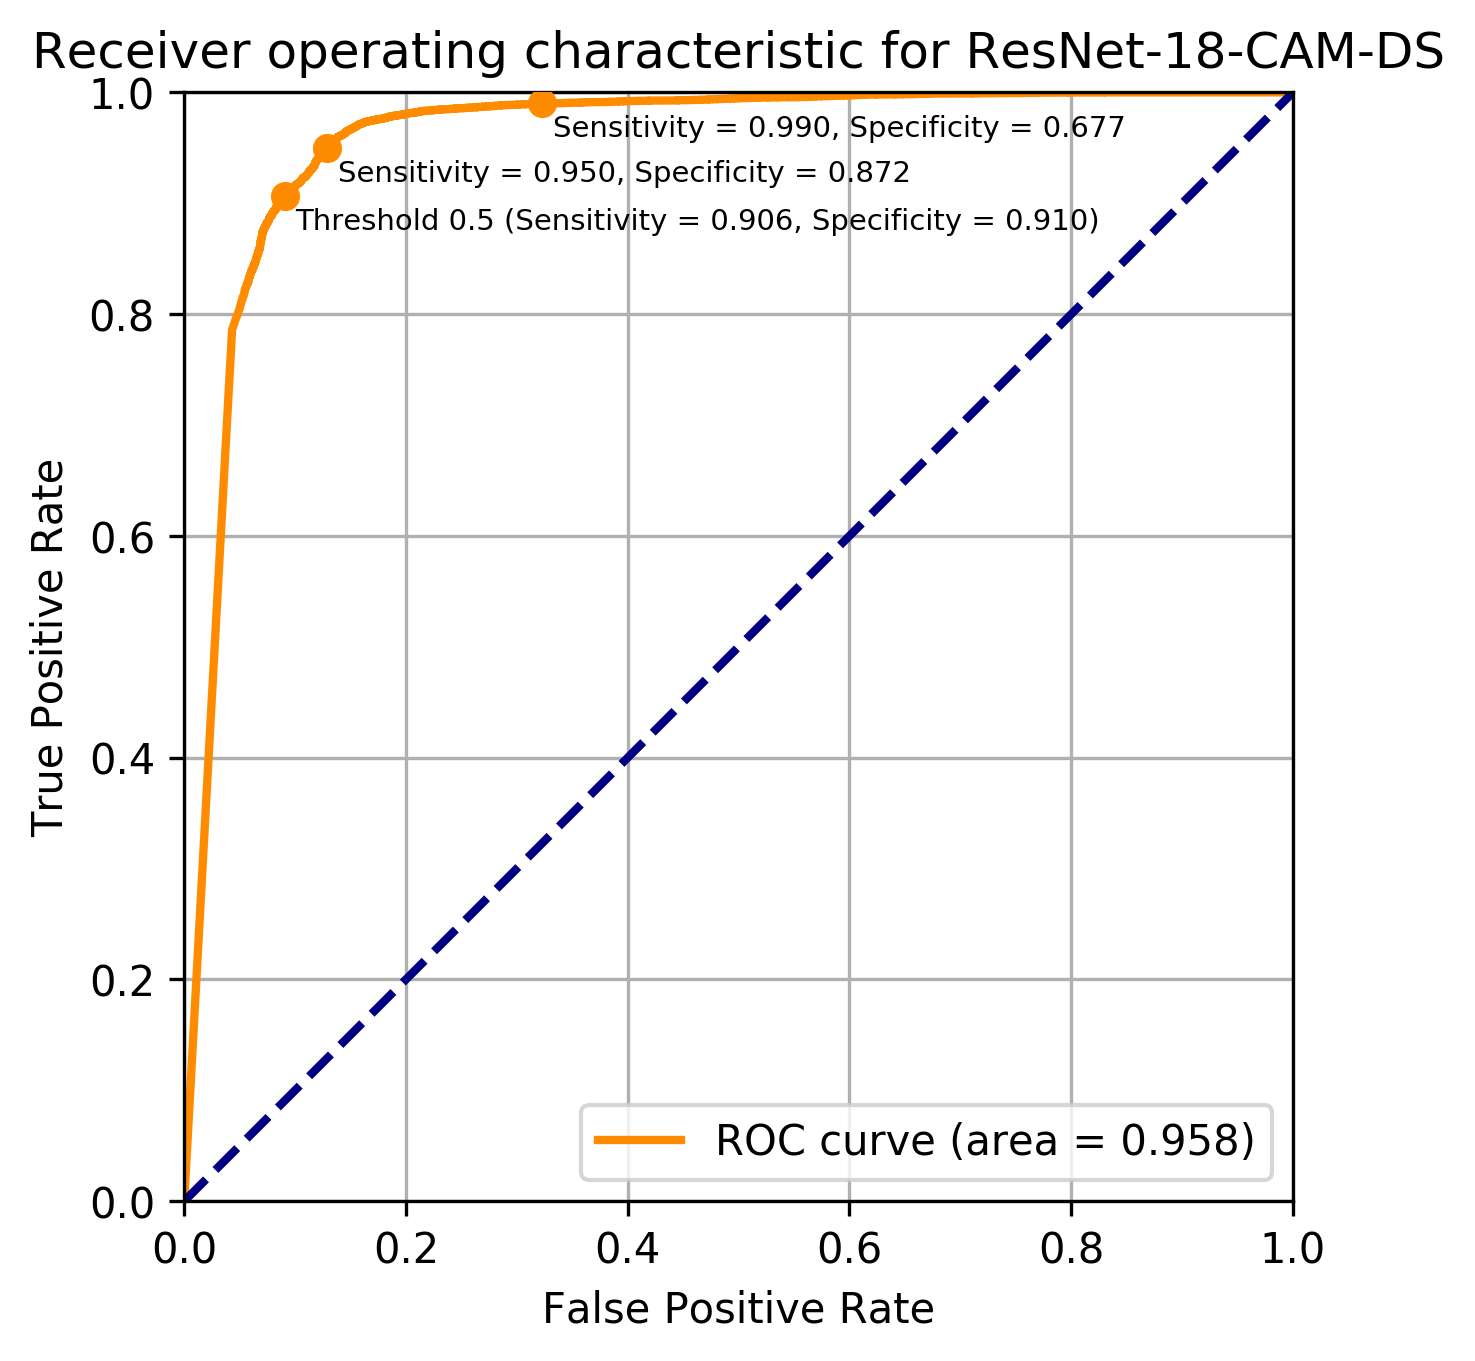}
	\caption{ROC curve based on the ResNet-18-CAM-DS predictions. Frames belonging to the testing set of all the folds were considered (although predictions for each fold were estimated with the network trained for such fold). As our system is intended to be used as a CADe, operating points at a sensitivity of \SI{95}{percent} and \SI{99}{percent} are shown for illustrative purposes.}
	\label{fig:roc_resnet_18_cam_ds}
\end{figure*}
